# Supplementary material for: MULDEF: Multi-model-based Defense Against Adversarial Examples for Neural Networks
Source: arXiv:1809.00065 source file (2019-07-27)
Supplement: Supplementary file 1 [file appendix.tex]

\begin{appendix}

 \begin{table}[h]
   
     \centering
     \begin{tabular}{*{1}{|>{\centering\arraybackslash}p{0.23\columnwidth}}*{5}{|>{\centering\arraybackslash}p{0.08\columnwidth}}|}
         \hline
         \multirow{2}{*}{\textbf{Models}}   & \multicolumn{5}{c|}{\textbf{Accuracy on adversarial examples}}  \\ \cline{2-6}
         & \textbf{$Adv_T$} & \textbf{$Adv_{M_1}$} & \textbf{$Adv_{M_2}$} & \textbf{$Adv_{M_3}$} & \textbf{$Adv_{M_4}$}   \\ \hline
         \textbf{$T$}      & 14.47\%  & 57.10\%  & 52.89\% & 50.98\% & 49.91\% \\ \hline
         \textbf{$M_1$}    & \textbf{65.22\%}  & 14.62\%  & 73.14\% & 60.53\% & 58.04\% \\ \hline
         \textbf{$M_2$}    & 58.30\%  & \textbf{72.82\%}  & 13.71\% & 67.72\% & 57.01\% \\ \hline
         \textbf{$M_3$}    & 59.17\%  & 60.97\%  & \textbf{71.07\%} & 19.27\% & \textbf{64.86\%} \\ \hline
         \textbf{$M_4$}    & 61.64\%  & 62.10\%  & 65.79\% & \textbf{68.46\%} & 20.85\% \\ \hline
     \end{tabular}
     \caption{Accuracy of each model in \toolName against FGSM with 5 models on each adversarial example set for CIFAR-10. The highest accuracy for each adversarial example set is marked in \textbf{bold}.}
     \label{fig:fgsm-cifar-modelaccuraies}
 \end{table}

 \begin{table}[h]

     \centering
     \begin{tabular}{*{1}{|>{\centering\arraybackslash}p{0.23\columnwidth}}*{5}{|>{\centering\arraybackslash}p{0.08\columnwidth}}|}
         \hline
         \multirow{2}{*}{\textbf{Models}}   & \multicolumn{5}{c|}{\textbf{Accuracy on adversarial examples}}  \\ \cline{2-6}
         & \textbf{$Adv_T$} & \textbf{$Adv_{M_1}$} & \textbf{$Adv_{M_2}$} & \textbf{$Adv_{M_3}$} & \textbf{$Adv_{M_4}$}   \\ \hline
         \textbf{$T$}      & 00.00\%  & 74.95\%  & 62.48\% & 59.13\% & 66.71\% \\ \hline
         \textbf{$M_1$}    & 97.10\%  & 00.00\%  & 90.94\% & 76.51\% & 79.54\% \\ \hline
         \textbf{$M_2$}    & 97.51\%  & 96.70\%  & 00.00\% & 91.81\% & 86.67\% \\ \hline
         \textbf{$M_3$}    & 97.94\%  & 96.80\%  & 96.63\% & 00.00\% & \textbf{93.94\%} \\ \hline
         \textbf{$M_4$}    & \textbf{98.37\%}  & \textbf{97.58\%}  & \textbf{96.83\%} & \textbf{96.50\%} & 00.00\% \\ \hline
     \end{tabular}
     \caption{Accuracy of each model in \toolName against C\&W with 5 models on each adversarial example set for MNIST. The highest accuracy for each adversarial example set is marked in \textbf{bold}.}
     \label{fig:cw-mnist-modelaccuraies}
 \end{table}

 \begin{table}[h]
   
     \centering
     \begin{tabular}{*{1}{|>{\centering\arraybackslash}p{0.23\columnwidth}}*{5}{|>{\centering\arraybackslash}p{0.08\columnwidth}}|}
         \hline
         \multirow{2}{*}{\textbf{Models}}   & \multicolumn{5}{c|}{\textbf{Accuracy on adversarial examples}}  \\ \cline{2-6}
         & \textbf{$Adv_T$} & \textbf{$Adv_{M_1}$} & \textbf{$Adv_{M_2}$} & \textbf{$Adv_{M_3}$} & \textbf{$Adv_{M_4}$}   \\ \hline
         \textbf{$T$}      & 00.00\%  & 72.43\%  & 74.90\% & 74.99\% & 76.16\% \\ \hline
         \textbf{$M_1$}    & 75.12\%  & 00.00\%  & 74.63\% & 74.25\% & 74.77\% \\ \hline
         \textbf{$M_2$}    & 78.00\%  & 77.57\%  & 00.00\% & 77.70\% & 77.88\% \\ \hline
         \textbf{$M_3$}    & 77.30\%  & 76.21\%  & 76.84\% & 00.00\% & \textbf{76.95\%} \\ \hline
         \textbf{$M_4$}    & \textbf{79.24\%}  & \textbf{78.29\%}  & \textbf{78.61\%} & \textbf{78.60\%} & 00.02\% \\ \hline
     \end{tabular}
     \caption{Accuracy of each model in \toolName against C\&W with 5 models on each adversarial example set for CIFAR-10. The highest accuracy for each adversarial example set is marked in \textbf{bold}.}
     \label{fig:cw-cifar-modelaccuraies}
 \end{table}

Tables VII, VIII, and IX (along with Table~\ref{fig:fgsm-mnist-modelaccuraies}) show the accuracy of each model in \toolName under different settings. For FGSM, each of the four models, $M_1, M_2, M_3, M_4$, is robust on different sets of adversarial examples. Their diversity provides robustness of our overall defense approach. For C\&W, the last model ($M_4$), which is trained with all the adversarial examples generated for the other models, is the most robust against $Adv_T, Adv_{M_1}, Adv_{M_2}, Adv_{M_3}$. However, \toolName still needs $M_3$ to help defend the adversarial examples for $M_4$ ($Adv_{M_4}$).

 \end{appendix}
